# Supplementary material for: Stability from activity
Source: arXiv:1711.02407 ancillary file (2017-11-07)
Supplement: Supplementary file 1 [file supp_pap.pdf]

# Stability from activity: Supplementary Information

Ananyo Maitra,[1,*] Pragya Srivastava,[2] M. Cristina Marchetti,[3]
Juho Lintuvuori,[4] Sriram Ramaswamy,[5] and Martin Lenz[1,†]

[1] *LPTMS, CNRS, Univ. Paris-Sud, Université Paris-Saclay, 91405 Orsay, France*
[2] *The Francis Crick Institute, Lincolns Inn Fields Laboratory, 44 Lincolns Inn Fields, London WC2A 3LY*
[3] *Physics Department and Syracuse Soft Matter Program, Syracuse University, Syracuse, NY 13244, USA*
[4] *Univ. Bordeaux, CNRS, LOMA, UMR 5798, F-33405 Talence, France*
[5] *Indian Institute of Science, Bangalore 560012, India*

We present a complete calculation of the linear stability of active nematic films on a substrate in section I including anisotropic mobilities and all possible active forces. We further explicitly calculate the concentration fluctuations and demonstrate that they indeed diverge at small wavevectors. In subsection I A we show that for incompressible systems on substrates a combination of anisotropic mobility and the standard active force is not sufficient to generate the velocity field anisotropy resulting from the second active force. In section I B we show that in a momentum conserved two-dimensional film even the combination of anisotropic viscosity and activity can not stabilise the ordered state which is generically unstable. Therefore, we demonstrate that the introduction of substrates in active systems lead to qualitatively different physical behaviour. In the next section, II we demonstrate that the two-dimensional dynamics we postulated, describe the effective equations for a three-dimensional fluid, confined in one direction, for lateral scales that are much larger compared to the scale of the confinement. In section III we briefly discuss the different scaling behaviour of the standard active term and the new one at large distances and show that the latter, which remains constant with scale, dominates over the former which vanishes with scale. Finally, in section IV we present a complete theory of living liquid crystals.

## I. LINEAR STABILITY ANALYSIS FOR GENERAL TWO-DIMENSIONAL INCOMPRESSIBLE ACTIVE NEMATICS

### A. Dynamics on a substrate

The most general free energy for small angular fluctuations of a two-dimensional nematic about a state ordered along the $\hat{x}$ direction is

$$\mathcal{H} = \int d^2\mathbf{r} \left[\frac{K_1}{2}(\partial_x\theta)^2 + \frac{K_2}{2}(\partial_y\theta)^2 + \gamma c \partial_x\partial_y\theta + f(c)\right] \tag{1}$$

where $K_1$ and $K_2$ are the standard bend and splay elastic constants, the $\gamma$ term is the most general coupling at the second order in gradients between angular and concentration fluctuations and $f(c)$ is an arbitrary function of concentration.

The equation for angular fluctuations reads, to linear order,

$$\partial_t\theta = \frac{1-\lambda}{2}\partial_x v_y - \frac{1+\lambda}{2}\partial_y v_x + \Gamma_\theta(K_1\partial_x^2\theta + K_2\partial_y^2\theta) - \Gamma_\theta\gamma\partial_x\partial_y c \tag{2}$$

The force balance equation with an anisotropic friction is

$$\Gamma_{ij}v_j = -\partial_i\Pi + f_i^a + f_i^p \tag{3}$$

where the passive force density has the same expression as in the main text

$$\mathbf{f}^p = -\frac{1+\lambda}{2}\partial_y\left(\frac{\delta\mathcal{H}}{\delta\theta}\right)\hat{\mathbf{x}} + \frac{1-\lambda}{2}\partial_x\left(\frac{\delta\mathcal{H}}{\delta\theta}\right)\hat{\mathbf{y}}. \tag{4}$$

and the active force density has an extra piece due to concentration fluctuations compared to the main text

$$f_x^a = -(\zeta_1\Delta\mu + \zeta_2\Delta\mu)\partial_y\theta + \zeta_3\Delta\mu\partial_x c \tag{5a}$$
$$f_y^a = -(\zeta_1\Delta\mu - \zeta_2\Delta\mu)\partial_x\theta - \zeta_3\Delta\mu\partial_y c, \tag{5b}$$

For symmetry reasons the friction matrix $\mathbf{\Gamma}$ in (3) has to be diagonal to zeroth order in the fields since it has to be constructed from the identity tensor or the apolar tensor characterising the orientational order along $\hat{x}$: $\hat{x}\hat{x} - (1/2)\mathsf{I}$, where $\mathsf{I}$ is the unit tensor. Thus, the mobility $\mathsf{M} = \mathbf{\Gamma}^{-1}$ is also diagonal and can be written as

$$\mathsf{M} = \begin{pmatrix} m_1 & 0 \\ 0 & m_2 \end{pmatrix} \tag{6}$$

where $m_1$ and $m_2$ are arbitrary coefficients. Writing $\mathbf{f} = \mathbf{f}^p + \mathbf{f}^a$, and Fourier transforming Eq.(3), we get

$$v_i = -iM_{ij}q_j\Pi + M_{ij}f_j. \tag{7}$$

Incompressibility yields

$$iq_iv_i = 0 = q_iM_{ij}q_j\Pi + iq_iM_{ij}f_j. \tag{8}$$

Thus,

$$\Pi = -i\frac{q_lM_{lm}f_m}{q_nM_{np}q_p}. \tag{9}$$

With this, Eq.(7) can be written as

$$v_i = -M_{ij}\frac{q_jq_lM_{lm}f_m}{q_nM_{np}q_p} + M_{ij}\delta_{jm}f_m = M_{ij}\left[\delta_{jm} - \frac{q_jq_lM_{lm}}{q_nM_{np}q_p}\right]f_m \tag{10}$$

Inserting Eqs. (4), (5) and (10) into the space-time Fourier-transformed version of Eq. (2), we obtain

$$-i\omega\theta = -q^2\left[\frac{\Delta\mu m_1m_2(1-\lambda\cos 2\phi)(\zeta_2 - \zeta_1\cos 2\phi)}{2(m_1\cos^2\phi + m_2\sin^2\phi)} + \Gamma_\theta K(\phi)\right]\theta + q^2\sin 2\phi\left[\frac{\zeta_3\Delta\mu m_1m_2(1-\lambda\cos 2\phi)}{2(m_1\cos^2\phi + m_2\sin^2\phi)} + \frac{\Gamma_\theta\gamma}{2}\right]\delta c \tag{11}$$

where $\delta c$ describes fluctuations away from the steady state value of the concentration $c = c_0$, $\phi$ is the angle between the wavevector direction and $\hat{x}$ and

$$K(\phi) = K_1\cos^2\phi + K_2\sin^2\phi. \tag{12}$$

For $m_1 = m_2 = 1/\Gamma$ and $\gamma = \zeta_3 = 0$, we recover Eq.(7) of the main text. We also see from (11) that if $\zeta_2 = 0$, the mere fact that $m_1 \neq m_2$ can not prevent an instability either just above or just below $\phi = \pi/4$ for sufficiently high $\Delta\mu$. This implies that in an incompressible system, the new active force can not be viewed simply as arising due to an anisotropic mobility component but instead has to be viewed as a new source of nonequilibrium forcing. In other words, the Poisson bracket between $\mathbf{v}$ and the chemical coordinate whose field is $\Delta\mu$ has to have an extra symmetry-allowed piece in systems that do not conserve angular momentum. This distinction does not arise for compressible systems.

The concentration fluctuation equation is

$$\partial_t c = -\nabla\cdot(\mathbf{J}^p + \mathbf{J}^a). \tag{13}$$

We take the passive current to be isotropic

$$\mathbf{J}^p = -D_c\nabla c \tag{14}$$

while the active current has the form

$$\mathbf{J}^a = -\Delta\mu[(\zeta_{cx}\partial_x c + \zeta_c\partial_y\theta)\hat{x} + (\zeta_{cy}\partial_y c + \zeta_c\partial_x\theta)\hat{y}]. \tag{15}$$

We had only considered the angle-dependent part of the concentration current in the main text.

We now define

$$D(\phi) = \left[\frac{\Delta\mu m_1m_2(1-\lambda\cos 2\phi)(\zeta_2 - \zeta_1\cos 2\phi)}{2(m_1\cos^2\phi + m_2\sin^2\phi)} + \Gamma_\theta K(\phi)\right] \tag{16}$$

$$\gamma_c(\phi) = -\sin 2\phi\left[\frac{\zeta_3\Delta\mu m_1m_2(1-\lambda\cos 2\phi)}{2(m_1\cos^2\phi + m_2\sin^2\phi)} + \frac{\Gamma_\theta\gamma}{2}\right] \tag{17}$$

$$D_m(\phi) = D_c + \Delta\mu\left(\frac{\zeta_{cx}+\zeta_{cy}}{2} + \frac{\zeta_{cx}-\zeta_{cy}}{2}\cos 2\phi\right) \tag{18}$$

$$\Upsilon(\phi) = \sin 2\phi \frac{\zeta_c \Delta\mu}{2}. \tag{19}$$

We can now calculate the eigenfrequencies of the coupled dynamics of $\theta$ and $\delta c$:

$$\omega_\pm = -i\Xi_\pm q^2 \tag{20}$$

where

$$\Xi_\pm = \frac{1}{2}\left[D(\phi) + D_m(\phi) \pm \sqrt{\{D(\phi) - D_m(\phi)\}^2 + 4\gamma_c(\phi)\Upsilon(\phi)}\right] \tag{21}$$

For large $\Delta\mu$ for both eigenvalues to be stabilising, in addition to the conditions in the main text, we require the isotropic diffusivity to be at least as large as the anisotropic one , $(\zeta_{cx} - \zeta_{cy}) \leq (\zeta_{cx} + \zeta_{cy})$, and

$$D(\phi)D_m(\phi) > \gamma_c(\phi)\Upsilon(\phi), \tag{22}$$

when only the $\Delta\mu$ dependent parts of $D(\phi)$, $D_m(\phi)$ and $\gamma_c(\phi)$ are retained, for all $\phi$. For $\zeta_c$ and $\zeta_3$ having opposite signs, this requires $\zeta_c\zeta_3 \ll (\zeta_{cx}+\zeta_{cy})(\zeta_2-\zeta_1)$. The ordered phase remains stable when $\zeta_c$ and $\zeta_3$ have the same sign. However, in this case, when $|\gamma_c(\phi)\Upsilon(\phi)| > [D(\phi) - D_m(\phi)]^2$ the eigenvalues acquire an imaginary part implying the existence of wavelike excitations with a $\omega \sim q^2$ spectrum. Note that these are not the standard wave excitations present in passive nematics at low damping. Those have already been eliminated by assuming an overdamped dynamics for the velocity field. These are, instead, the analogues of the Toner-Tu waves [1] in our apolar system.

With these eigenfrequencies in hand, we can calculate the equal-time correlators of the concentration field in the ordered phase. For this we add a Gaussian, zero-mean nonconserving noise $\xi_\theta(\mathbf{r}, t)$ to Eq. (2) with the correlator

$$\langle \xi_\theta(\mathbf{r}, t)\xi_\theta(\mathbf{r}', t')\rangle = B_\theta \delta(\mathbf{r} - \mathbf{r}')\delta(t - t'). \tag{23}$$

We should also add a conserving noise $\xi_c(\mathbf{r}, t)$ to (13) but that only leads to a higher order in wavevector correction to the equal-time concentration correlations and is irrelevant in the $q \to 0$ limit we are interested in. Using Eqs. (11), (13)-(15) and (21), we find the Fourier-transformed concentration fluctuations

$$\delta c(\mathbf{q}, \omega) = \frac{\Upsilon(\phi) q^2 \xi_\theta}{(\omega + i\Xi_+ q^2)(\omega + i\Xi_- q^2)} \tag{24}$$

Autocorrelating this, we find

$$\langle |\delta c(\mathbf{q}, \omega)|^2\rangle = \frac{\Upsilon(\phi)^2 q^4 B_\theta}{(\omega^2 + \Xi_+^2 q^4)(\omega^2 + \Xi_-^2 q^4)} \tag{25}$$

From this, we can calculate the equal-time correlator as

$$\langle \delta c(\mathbf{q}, t)\delta c(-\mathbf{q}, t)\rangle = \int_{-\infty}^{\infty} \frac{d\omega}{2\pi}\langle |\delta c(\mathbf{q}, \omega)|^2\rangle = \frac{\Upsilon(\phi)^2 q^4 B_\theta}{2q^6(\Xi_+\Xi_-)(\Xi_+ + \Xi_-)} \propto \frac{1}{q^2}. \tag{26}$$

As we discussed in the main text, this $1/q^2$ divergence of the static structure factor leads to giant number fluctuations in our system notwithstanding the presence of incompressible solvent dynamics.

### B. Momentum conserving dynamics in the absence of a substrate

In this section we show that anisotropic viscosity cannot mimic the effect of the second activity constant in a momentum conserved system. For a momentum conserved two-dimensional active fluid, $\zeta_2 = 0$ and $\zeta_3$ and $\zeta_1$ are related to each other since they both arise from the divergence of an active stress

$$\boldsymbol{\sigma}^{act} = -\zeta_1 \alpha(c)\mathbf{Q} \tag{27}$$

where $\alpha(c)$ is an arbitrary function of concentration and

$$\mathbf{Q} = \frac{S}{2}\begin{pmatrix}\cos 2\theta & \sin 2\theta \\ \sin 2\theta & -\cos 2\theta\end{pmatrix} \tag{28}$$

is the nematic order parameter, whose magnitude $S$ can be taken to be fixed at a constant value which we rescale to 1 without loss of generality. Further, the damping matrix $\Gamma_{ij}$ is now $\propto q^2$. The most general viscosity tensor for a two-dimensional incompressible nematogenic fluid can be written as

$$\boldsymbol{\sigma}^{vis} = \eta_0 \mathbf{U} + \eta_1 \mathbf{Q}^0(\mathbf{Q}^0 : \mathbf{U}), \tag{29}$$

where $\mathbf{U}$ is the symmetrised velocity gradient tensor and $\mathbf{Q}^0 = \hat{x}\hat{x} - (1/2)\mathbf{I}$ is the apolar order parameter corresponding to a state ordered along the $\hat{x}$ direction. Note there is no contribution of the form $\mathbf{Q}^0 \cdot \mathbf{U}$ in the viscous stress since the symmetrised traceless part of $\mathbf{Q}^0 \cdot \mathbf{U}$ is identically 0. Taking the divergence of the viscous tensor, we get the viscous force

$$\nabla \cdot \boldsymbol{\sigma}^{vis} = [\eta_0 \nabla^2 v_x + \eta_1(\partial_x^2 v_x - \partial_x \partial_y v_y)]\hat{x} + [\eta_0 \nabla^2 v_y + \eta_1(\partial_y^2 v_y - \partial_x \partial_y v_y)]\hat{y} \tag{30}$$

Using incompressibility $\partial_x v_x = -\partial_y v_y$, we get

$$\nabla \cdot \boldsymbol{\sigma}^{vis} = (\eta_0 \nabla^2 + 2\eta_1 \partial_x^2) v_x \hat{x} + (\eta_0 \nabla^2 + 2\eta_1 \partial_y^2) v_y \hat{y} \tag{31}$$

Thus, the mobility coefficients equivalent to (6) are

$$m_1 = \frac{1}{\eta_0 q^2 + 2\eta_1 q_x^2} = \frac{1}{q^2(\eta_0 + 2\eta_1 \cos^2\phi)} \tag{32}$$

$$m_2 = \frac{1}{\eta_0 q^2 + 2\eta_1 q_y^2} = \frac{1}{q^2(\eta_0 + 2\eta_1 \sin^2\phi)} \tag{33}$$

This implies that

$$\frac{m_1 m_2}{2(m_1 \cos^2\phi + m_2 \sin^2\phi)} = \frac{1}{q^2}\frac{1}{\eta_0 + \eta_1 - \eta_1 \cos 4\phi} \tag{34}$$

This leads to the dispersion relation for angular fluctuations, which to zeroth order in wavevectors, and rescaling $c_0 = 1$, reads

$$-i\omega\theta = \frac{\Delta\mu\zeta_1 \cos 2\phi(1 - \lambda\cos 2\phi)}{\eta_0 + \eta_1 - \eta_1 \cos 4\phi}\theta \tag{35}$$

The right hand side of this equation is positive either just below or just above $\phi = \pi/4$ depending on the sign of $\zeta_1$ implying that despite the inclusion of anisotropic viscosity the system is always unstable irrespective of parameter values.

## II. DERIVATION OF EFFECTIVE TWO-DIMENSIONAL EQUATIONS OF MOTION FROM THREE-DIMENSIONAL EQUATIONS FOR ACTIVE FLUIDS CONFINED IN ONE DIRECTION

In this section we derive the effective equations for a suspension of apolar filaments, endowed with active stresses, in a fluid confined between two parallel plates separated by a distance $h$. We assume that the two plates impose perpendicular anchoring conditions on the filaments, no-slip, no-penetration boundary conditions on the velocity field and no-flux boundary condition on the concentration field. We start with the standard three-dimensional equations for the number density $\bar{c}(\bar{\mathbf{x}}, t)$, the traceless symmetric three-dimensional orientation tensor $\bar{\mathbf{Q}}(\bar{\mathbf{x}}, t)$ of the filaments and the velocity field $\bar{\mathbf{v}}(\bar{\mathbf{x}}, t) = (\bar{\mathbf{v}}_\perp, \bar{v}_z)$, as functions of three-dimensional position $\bar{\mathbf{x}}$ and time $t$. We then average over the thickness of the film to get effective equations of motion valid for in-plane scales $L \gg h$.

The density of filaments follows the conservation law

$$\partial_t \bar{c} = \bar{\nabla} \cdot [\bar{c}\bar{\zeta}_c \Delta\mu \bar{\nabla} \cdot (\bar{c}\bar{\mathbf{Q}}) + \bar{D}_c \bar{\nabla}\bar{c} + \bar{D}_{cQ}\bar{\mathbf{Q}} \cdot \bar{\nabla}\bar{c}]. \tag{36}$$

with $\bar{\zeta}_c$ and $\bar{D}_c$ and $\bar{D}_{cQ}$ governing active and diffusive fluxes respectively. The $\bar{D}_{cQ}$ is the passive coefficient for anisotropic diffusivity. Anisotropic diffusivity arises, in addition, from the active flux encoded by the first term in the R.H.S. of (36). $\bar{\nabla}$ denotes three-dimensional derivatives. The equation of motion

$$\partial_t \bar{\mathbf{Q}} + \bar{\mathbf{v}} \cdot \bar{\nabla} \bar{\mathbf{Q}} = -\bar{\lambda} \bar{\mathbf{U}} + \bar{\lambda}_1 (\bar{\mathbf{U}} \bar{\mathbf{Q}})^{ST} - \bar{\mathbf{Q}} \cdot \bar{\boldsymbol{\omega}} + \bar{\boldsymbol{\omega}} \cdot \bar{\mathbf{Q}} - \bar{\boldsymbol{\Gamma}}_Q \bar{\mathbf{H}}. \tag{37}$$

for the orientational order parameter is taken to have the same form as in passive systems [2] where the superscript $ST$ on a tensor denotes its symmetric traceless part. This assumption in principle introduces a restriction in the dynamics through a relation [3] between the coefficients of terms of the form $\bar{\nabla} \bar{\mathbf{Q}} \bar{\nabla} \bar{\mathbf{Q}}$ and $\bar{\mathbf{Q}} \bar{\nabla} \bar{\nabla} \bar{\mathbf{Q}}$ in (37), as both arise through the molecular field

$$\bar{\mathbf{H}} = \left( \frac{\delta \bar{\mathcal{H}}}{\delta \bar{\mathbf{Q}}} \right)^{ST} \tag{38}$$

obtained from the Landau-de-Gennes free-energy functional $\bar{\mathcal{H}} = \int d\bar{\mathbf{x}} \bar{\mathfrak{h}}$,

$$\bar{\mathfrak{h}} = \bar{A} \bar{\mathbf{Q}}^2 + \bar{B} \bar{\mathbf{Q}} : (\bar{\mathbf{Q}} \cdot \bar{\mathbf{Q}}) + \bar{C} (\bar{\mathbf{Q}} : \bar{\mathbf{Q}}) \bar{\mathbf{Q}}^2 + \frac{\bar{K}_1}{2} (\bar{\nabla} \bar{\mathbf{Q}})^2 + \frac{\bar{K}_2}{2} (\bar{\nabla} \cdot \bar{\mathbf{Q}})^2 + \frac{\bar{K}_3}{2} \bar{\mathbf{Q}} : (\bar{\nabla} \bar{\mathbf{Q}} : \bar{\nabla} \bar{\mathbf{Q}}) + \bar{\gamma} \bar{\nabla} \bar{\nabla} \bar{c} : \bar{\mathbf{Q}}, \tag{39}$$

which includes a symmetry-allowed coupling $\bar{\gamma}$ between the concentration and the apolar order-parameter [4]. However, (a) the role of such restriction is unimportant in our linearised treatment and (b) flows induced by active stresses enter Eq.(37) through flow-alignment terms proportional to $\bar{\lambda}$ and $\bar{\lambda}_1$. In Eq.(37), $\bar{\mathbf{U}}$ and $\bar{\boldsymbol{\omega}}$ are respectively the symmetric and the anti-symmetric parts of the velocity gradient tensor $(\bar{\nabla} \bar{\mathbf{v}})$.

The velocity, as appropriate for the slow flows we are interested in, is taken to obey the Stokes equation $\bar{\nabla} \cdot \bar{\boldsymbol{\sigma}} = 0$, where the stress $\bar{\boldsymbol{\sigma}}$ is the sum of the active and the passive stress. The passive stress is

$$\bar{\boldsymbol{\sigma}}^p = 2\bar{\eta} \bar{\mathbf{U}} - \bar{\Pi} \bar{\mathbf{I}} - \bar{\lambda} \bar{\mathbf{H}} + \bar{\lambda}_1 (\bar{\mathbf{Q}} \bar{\mathbf{H}})^{ST} - 2(\bar{\mathbf{Q}} \bar{\mathbf{H}})^A - \bar{\nabla} \bar{\mathbf{Q}} : \frac{\bar{\partial} \bar{\mathfrak{h}}}{\bar{\partial} (\bar{\nabla} \bar{\mathbf{Q}})}, \tag{40}$$

with the isotropic viscosity $\bar{\eta}$ (we neglect anisotropic viscosity for clarity), a pressure $\bar{\Pi}$ determined by three-dimensional incompressibility and with $\bar{\mathfrak{h}}$ representing the free-energy density. The active part of the stress is given by

$$\bar{\sigma}^a_{ij} = \Delta\mu [\bar{\zeta}_0 \bar{\delta}_{ij} - \bar{\zeta}_1 \bar{Q}_{ij} - \bar{\zeta}_2 \{ \bar{\partial}_i (\bar{Q}_{jk} \bar{\partial}_m \bar{Q}_{mk}) + \bar{\partial}_j (\bar{Q}_{ik} \bar{\partial}_m \bar{Q}_{mk}) \}]. \tag{41}$$

The coefficients of the active stresses should, in principle, be taken to be proportional to the local concentration of active filaments. Note that all of these terms arise as off-diagonal reactive couplings between the velocity and the chemical potential difference between the fuel and its reaction products, $\Delta\mu$, and thus, have no counterparts in the equation for $\bar{\mathbf{Q}}$. The term proportional to $\bar{\zeta}_2$, while in principle present in theories of bulk active fluids, is not generally explicitly considered since in those theories it is subdominant to the active forcing entering at a lower order in gradient through the term proportional to $\bar{\zeta}_1$. However, in our thickness-averaged description, the gradients along the $z$ direction are of order $\sim 1/h$ and this term will end up contributing at the same order in $L$ as the term proportional to $\bar{\zeta}_1$. This term, along with all other terms at the same order in gradients can, in principle, be obtained by expanding a general active force density à la Ref. [5] to third order in gradients. Other active terms at this or higher order in gradients do not introduce any qualitatively new effect in the thickness-averaged equation of motion. For instance, another possible term in the active stress is $\bar{\nabla}_i \bar{\nabla}_k \bar{Q}_{jk} + \bar{\nabla}_j \bar{\nabla}_k \bar{Q}_{ik}$ which, in the thickness-averaged description, leads to an active force of the same form as the one arising from the term with the coefficient $\bar{\zeta}_1$ in (41).

We now supplement these equations with the boundary conditions mentioned at the beginning of the section and integrate over the thickness to find an effective set of two-dimensional equations. For this, we use a lubrication approximation, standard in the study of thin-film flows [6], in which terms in the equations of motion at higher orders in $\varepsilon = h/L$ are discarded. The incompressibility condition, $\bar{\nabla} \cdot \bar{\mathbf{v}} = 0$ upon scaling $z$ by $h$ and $x$ and $y$ by $L$ reads $\varepsilon \bar{\nabla}_\perp \cdot \bar{\mathbf{v}}_\perp + \bar{\partial}_z \bar{v}_z = 0$. To order $\varepsilon^0$, this yields $\bar{\partial}_z \bar{v}_z = 0$ implying $\bar{v}_z$ is independent of $z$. Due to the no-penetration boundary condition in the $z$ direction, this implies $\bar{v}_z = 0$ at this order. As is also clear from this, in the lubrication approximation, $\bar{\partial}_z \gg \bar{\partial}_x, \bar{\partial}_y$ and hence, $\bar{\partial}_z^2 \gg \bar{\partial}_x^2, \bar{\partial}_y^2$. Assuming for simplicity a Poiseuille profile with a given mid-plane horizontal velocity $\bar{\mathbf{v}}_0$ and no slip on the bounding surfaces at $z = 0$ and $z = h$ we get an in-plane velocity

$$\bar{\mathbf{v}}_\perp(z) = \frac{4}{h^2} \bar{\mathbf{v}}_0 (zh - z^2). \tag{42}$$

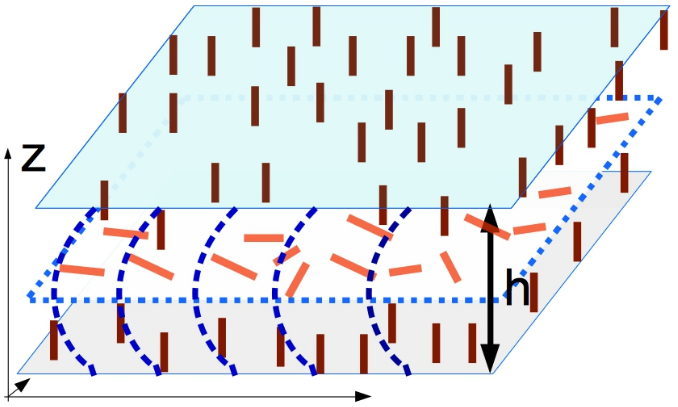


FIG. 1. Nematic fluid confined between two parallel plates separated by a distance $h$. The dark red bars show the anchoring of the nematogens at the top and the bottom surface. The orange bars show the orientation of the nematogens at a mid-plane outlined in light blue. The profile of the in-plane component (specifically the $Q_{xx}$ component) of the apolar tensor is schematically shown in dark blue. The active force with the coefficient $\zeta_2$ ultimately arises from the variation of the planar nematic curvature along the $z$ direction. The $z$-variation of the planar nematic curvature has different values along and transverse to the principal axis of the planar nematogenic order, leading to Eq. (**??**).

Thus, the $z$-averaged viscous force density is $(8\bar{\eta}/h^2)\bar{\mathbf{v}}_0$ and the $z$-averaged velocity is $\mathbf{v} = (2/3)\bar{\mathbf{v}}_0$, and

$$\frac{1}{h}\int_0^h \bar{\eta}\bar{\nabla}^2\bar{\mathbf{v}}_\perp dz = -\Gamma\mathbf{v} + O(\epsilon^2), \tag{43}$$

where

$$\Gamma = 12\bar{\eta}/h^2. \tag{44}$$

Though we have assumed a Poiseuille profile for the flow, only the numerical coefficient in the definition of $\Gamma$ can change if other kinds of flows (for instance, plug flow) are considered.

We now have to carry out a similar analysis for $\bar{\mathbf{Q}}$. The planar components of $\bar{\mathbf{Q}}$, $\bar{\mathbf{Q}}_{\perp\perp}$ have a non-trivial $z$-dependence, either because of boundary conditions directly (parallel anchoring on one plate and perpendicular anchoring on the other, for instance) or due to the presence of a mean-flow for $h > \sqrt{\bar{K}_Q\bar{\eta}/(\bar{\zeta}_1\Delta\mu)}$. Therefore, for any vector function $\bar{\mathbf{g}}(\bar{\nabla}, \bar{\mathbf{Q}})$ which may be composed of $\bar{\nabla}$ and $\bar{\mathbf{Q}}$,

$$\frac{1}{h}\int_0^h \bar{\nabla}^2\bar{\mathbf{g}}(\bar{\nabla}, \bar{\mathbf{Q}})dz \propto \frac{1}{h^2}\mathbf{g}(\nabla, \mathbf{Q}) \tag{45}$$

in analogy with (43), where $\bar{\mathbf{Q}}$, $\mathbf{g}(\nabla, \mathbf{Q})$ is its $z$-averaged value depending on $\mathbf{Q}$ – the $z$-averaged value of $\bar{\mathbf{Q}}$ projected onto the $xy$ plane – and the two-dimensional gradient operator $\nabla$. Now, taking the divergence of the term proportional to $\bar{\zeta}_2$, we see that it yields a term $\bar{\nabla}^2(\bar{Q}_{ik}\bar{\nabla}_m\bar{Q}_{km})$ and another one which is a total gradient and simply modifies the pressure. Upon averaging over the thickness, $\bar{\nabla}^2(\bar{Q}_{ik}\bar{\nabla}_m\bar{Q}_{km})$ leads to a force $f_i^a \propto (1/h^2)Q_{ik}\nabla_m Q_{km}$ in the lubrication approximation. The proportionality constant depends on the details of the $z$-profile of the apolar tensor. In parallel with the argument presented for the velocity field, if we assume that $\bar{\mathbf{Q}}_{\perp\perp}\cdot(\bar{\nabla}_\perp\cdot\bar{\mathbf{Q}}_{\perp\perp})$, has a mid-plane value $[\bar{\mathbf{Q}}_{\perp\perp}\cdot(\bar{\nabla}_\perp\cdot\bar{\mathbf{Q}}_{\perp\perp})]^0$, and assume a simple parabolic profile for its $z$-dependence, which has to go to 0 at $z = 0$ and $z = h$ since there is no in-plane gradient of $\bar{\mathbf{Q}}$ at either surface, we obtain

$$[\bar{\mathbf{Q}}_{\perp\perp}\cdot(\bar{\nabla}_\perp\cdot\bar{\mathbf{Q}}_{\perp\perp})](z) = \frac{4}{h^2}[\bar{\mathbf{Q}}_{\perp\perp}\cdot(\bar{\nabla}_\perp\cdot\bar{\mathbf{Q}}_{\perp\perp})]^0 z(h-z). \tag{46}$$

Further replacing $z$-averages of products of fields, by products of averages, we obtain the proportionality constant $18\bar{\zeta}_2/h^2$ which implies that $\zeta_2$ in (**??**) is $9\bar{\zeta}_2/h^2$. Performing this exercise for all the other terms, we obtain the $z$-averaged Stokes equation

$$\Gamma\mathbf{v} = -\nabla\Pi - \lambda\nabla\cdot\mathbf{H} - 2\nabla\cdot(\mathbf{QH})^A - \zeta_1\Delta\mu\nabla\cdot\mathbf{Q} - 2\zeta_2\Delta\mu\mathbf{Q}\cdot(\nabla\cdot\mathbf{Q}). \tag{47}$$

where the effective pressure $\Pi = \frac{1}{h}\int_0^h dz\bar{\Pi}$ imposes the $z$-averaged incompressibility condition $\nabla_\perp \cdot \mathbf{v} = 0$, and $\mathbf{H}$ is the $z$-averaged value of $\bar{\mathbf{H}}$ projected onto the $xy$ plane. The dynamical equations for $\mathbf{Q}$ and the $z$-averaged concentration field $c$ are

$$\partial_t \mathbf{Q} = -\mathbf{v} \cdot \nabla \mathbf{Q} + \boldsymbol{\omega} \cdot \mathbf{Q} - \mathbf{Q} \cdot \boldsymbol{\omega} - \lambda \mathbf{U} - \Gamma_\theta \mathbf{H}, \tag{48}$$

where $\boldsymbol{\omega}$ and $\mathbf{U}$ denote the anti-symmetric and symmetric parts of the tensor $\nabla \mathbf{v}$, and

$$\partial_t c = \zeta_c \Delta\mu c_0^2 \nabla\nabla : (\mathbf{Q}) + (\zeta_c \Delta\mu c_0 + D_{cQ}) \nabla \cdot (\mathbf{Q} \cdot \nabla c) + D_c \nabla^2 c. \tag{49}$$

(47) and (48) are the equations (10) of the main text.

Note that these constitute a complete set of equation for two-dimensional incompressible active nematodynamics and can be used to study dynamics beyond the linear regime. In this context, a distinctive feature of active nematodynamics is the self-propulsion of $+1/2$ defects. This feature is unaffected by the inclusion of the new active force with the coefficient $\zeta_2$. Far from a defect, the magnitude of $\mathbf{Q}$ is constant, while the angle-field is $\theta = \pm n\psi/2$, where $n$ is any non-zero integer which describes the winding number, and $\psi$ is the azimuthal angle. The force generated by the term proportional to $\zeta_2$ due to this is $\propto n\hat{r}/r$, where $r$ is the radial distance of a point from the defect. Since this can be written as a gradient of a singular potential for all $n$ it can not lead to any flow in an incompressible system – it can be balanced by a pressure gradient. Thus, $\zeta_2$ by itself can not lead to propulsion of $+1/2$ defects but neither can it suppress the self-propulsion due to the active force $\nabla \cdot \mathbf{Q}$ as shown by [7, 8].

## III. BEYOND LINEAR THEORY: SCALING OF ACTIVE FORCE WITH DISTANCE

In this section we demonstrate that the standard active force with the coefficient $\zeta_1$ vanishes for large systems while the new active force does not. The reason for this is that active nematics have only quasi-long ranged order in two dimensions which implies that any anisotropy vanishes in the limit of infinite system size. Therefore, $\langle \cos 2\theta \rangle$ and $\langle \mathbf{Q} \rangle$ has to vanish as some typically small power $\eta$ of the system size i.e. $\langle \cos 2\theta \rangle \sim q^\eta$ in the limit $q \to 0$, where $q$ is the wavevector ($\langle \sin 2\theta \rangle$ is, of course, 0). As we show below, the $\zeta_1$ active force term is anisotropic and is associated with a factor $\cos 2\phi$, while the $\zeta_2$ active force term is isotropic. For clarity, we only consider a model with $\mathbf{v}$ and $\mathbf{Q}$ and no concentration. The coupled equations for the angle field and the velocity field, from eq (10) of the main text, are

$$\dot{\theta} = \frac{1 - \lambda \cos 2\theta}{2} \partial_x v_y - \frac{1 + \lambda \cos 2\theta}{2} \partial_y v_x + \Gamma_\theta K \nabla^2 \theta + \xi_\theta \tag{50}$$

$$\dot{\mathbf{v}} = -\Gamma \mathbf{v} - \nabla \Pi + \mathbf{f}^a + \boldsymbol{\xi}_\mathbf{v} \tag{51}$$

where $\xi_\theta$ and $\boldsymbol{\xi}_\mathbf{v}$ are Gaussian white noises and the active force from (47)

$$f_x^a = -\Delta\mu(\zeta_1 \cos 2\theta + \zeta_2) \partial_y \theta \tag{52}$$

$$f_y^a = -\Delta\mu(\zeta_1 \cos 2\theta - \zeta_2) \partial_x \theta \tag{53}$$

where, as before, we have taken the mean value of the order parameter magnitude $S$ to be 1. We only consider situations in which the ordered phase is stable. The length-scale dependence of $\langle \cos 2\theta \rangle$ immediately implies that both the effective flow-alignment parameter $\lambda$ and the effective active force coefficient $\zeta_1$, which in a self-consistent theory should be evaluated as $\langle \lambda \cos 2\theta \rangle$ and $\langle \zeta_1 \cos 2\theta \rangle$ respectively, has to run with scale with the exponent $\eta$ [9], while $\zeta_2$, which does not contain an anisotropic factor, does not vanish even in the limit of infinite systems. Using the analysis of Ref. [9] $\eta = B_\theta/(2\pi D_{\text{eff}})$ where $B_\theta$ is the strength of the noise $\xi_\theta$ and $D_{\text{eff}}$ is the isotropic part of the angular relaxation rate

$$D_{\text{eff}} = \Gamma_\theta K + \frac{\Delta\mu}{2\Gamma} [\zeta_2 + (\lambda \zeta_1)/2] \tag{54}$$

Thus, it is clear that the equations of motion for active nematics reduce to the equations of motion for active tetratics or hexatics, in which both $\lambda$ and $\zeta_1$ are 0 by symmetry, at large scales. Active nematics and hexatics however still have distinct number fluctuations statistics. If in addition we were to include the concentration dynamics, active concentration current of active nematic would also run with scale exactly as $\lambda$ or $\zeta_1$, but would leave its imprint in the concentration fluctuation, which would not reduce to those in hexatics, which scale as $q^0$ but would scale as $q^{(-2+2\eta)}$ as shown in Ref. [9]. The power-law vanishing of the active force with coefficient $\zeta_1$ while $\zeta_2$ remains constant implies that the latter dominates over the former at large scales.

## IV. LIVING LIQUID CRYSTALS

Living liquid crystals constitute [10] a new class of experimental active systems. They are composed of bacteria swimming in a passive nematic liquid crystal film. In this section we show that the effective dynamics of this system is described by our theory as well.

We start with a model with two different director fields, one for the passive nematic liquid-crystal, $\mathbf{N} = (\cos\Theta, \sin\Theta)$ and the other for the bacteria $\mathbf{n} = (\cos\theta, \sin\theta)$, where both are measured relative to the direction of ordering $\hat{\mathbf{x}}$, to decribe the thickness-averaged dynamics of the system. The coupled free energy is given by

$$\mathcal{H} = \int d^2\mathbf{r}\left[\frac{K_\Theta}{2}(\nabla\Theta)^2 + \frac{K_\theta}{2}(\nabla\theta)^2 - \cos^2(\Theta-\theta)\right] \tag{55}$$

The final term in the free-energy, which can be written as $-(\mathbf{N}\cdot\mathbf{n})^2$ in terms of the fields $\mathbf{N}$ and $\mathbf{n}$ describe the coupling between the directors. The equation of motion for director fields are

$$\dot{\theta} = \Gamma_\theta[\sin 2(\Theta-\theta) + K_\theta\nabla^2\theta] + \frac{1-\lambda_\theta}{2}\partial_x v_y - \frac{1+\lambda_\theta}{2}\partial_y v_x \tag{56}$$

$$\dot{\Theta} = \Gamma_\Theta[\sin 2(\theta-\Theta) + K_\Theta\nabla^2\Theta] + \frac{1-\lambda_\Theta}{2}\partial_x v_y - \frac{1+\lambda_\Theta}{2}\partial_y v_x \tag{57}$$

where $\Gamma_\theta$, $\lambda_\theta$, $\Gamma_\Theta$ and $\lambda_\Theta$ are the material parameters and $\mathbf{v}$ is the centre-of-mass velocity. Noting that only the bacteria generate active forces, the active force density is given as

$$f_x^a = -(\zeta_1\Delta\mu + \zeta_2\Delta\mu)\partial_y\theta \tag{58a}$$
$$f_y^a = -(\zeta_1\Delta\mu - \zeta_2\Delta\mu)\partial_x\theta, \tag{58b}$$

while the form of the passive force densities, completely specified by Onsager symmetry, are

$$\mathbf{f}^p = -\frac{1+\lambda_\theta}{2}\partial_y\left(\frac{\delta\mathcal{H}}{\delta\theta}\right)\hat{\mathbf{x}} + \frac{1-\lambda_\theta}{2}\partial_x\left(\frac{\delta\mathcal{H}}{\delta\theta}\right)\hat{\mathbf{y}} - \frac{1+\lambda_\Theta}{2}\partial_y\left(\frac{\delta\mathcal{H}}{\delta\Theta}\right)\hat{\mathbf{x}} + \frac{1-\lambda_\Theta}{2}\partial_x\left(\frac{\delta\mathcal{H}}{\delta\Theta}\right)\hat{\mathbf{y}}. \tag{59}$$

As usual, the overdamped equation for the velocity is given by

$$\Gamma\mathbf{v} = -\nabla\Pi + \mathbf{f}^p + \mathbf{f}^a. \tag{60}$$

Equations (55)-(60) completely specify the dynamics of living liquid crystals. We now study the linear stability of this system to small fluctuations. Eliminating the velocity by using transverse projector to enforce incompressibility, we obtain the coupled linear equations for $\theta$ and $\Theta$,

$$\dot{\theta}_q = 2\Gamma_\theta(\Theta_q-\theta_q) - \left[\Gamma_\theta K_\theta + \Delta\mu\frac{(1-\lambda_\theta\cos 2\phi)}{2\Gamma}(-\zeta_1\cos 2\phi+\zeta_2)\right]q^2\theta_q - \frac{(1-\lambda_\theta\cos 2\phi)}{2\Gamma}(\lambda_\Theta-\lambda_\theta)\cos 2\phi q^2(\theta_q-\Theta_q)$$
$$- \frac{(1-\lambda_\theta\cos 2\phi)^2}{4\Gamma}K_\theta q^4\theta_q - \frac{(1-\lambda_\theta\cos 2\phi)(1-\lambda_\Theta\cos 2\phi)}{4\Gamma}K_\Theta q^4\Theta_q \tag{61}$$

$$\dot{\Theta}_q = -2\Gamma_\Theta(\Theta_q-\theta_q) - \Gamma_\Theta K_\Theta q^2\Theta_q - \left[\Delta\mu\frac{(1-\lambda_\Theta\cos 2\phi)}{2\Gamma}(-\zeta_1\cos 2\phi+\zeta_2)\right]q^2\theta_q - \frac{(1-\lambda_\Theta\cos 2\phi)}{2\Gamma}(\lambda_\Theta-\lambda_\theta)\cos 2\phi q^2(\theta_q-\Theta_q)$$
$$- \frac{(1-\lambda_\Theta\cos 2\phi)^2}{4\Gamma}K_\Theta q^4\Theta_q - \frac{(1-\lambda_\theta\cos 2\phi)(1-\lambda_\Theta\cos 2\phi)}{4\Gamma}K_\theta q^4\theta_q \tag{62}$$

One of the two eigenvalues of this system of equations describes the fast relaxational dynamics of $(\mathbf{n}-\mathbf{N})$ at a rate $2(\Gamma_\Theta+\Gamma_\theta)$ while the other is the hydrodynamic mode corresponding to the broken rotation symmetry. Patterns are formed when this mode is unstable at leading order in wavevectors. The small wavevector growth-rate of the slow mode is given by $-i\omega = -w_1(\phi)q^2 - w_2(\phi)q^4$ where

$$w_1(\phi) = \left[\tilde{\Gamma}\tilde{K} + \frac{\Delta\mu}{2\Gamma}(1-\tilde{\lambda}\cos 2\phi)(-\zeta_1\cos 2\phi+\zeta_2)\right]. \tag{63}$$

Here, the renormalised material parameters are defined as

$$\tilde{\Gamma} = \frac{\Gamma_\theta \Gamma_\Theta}{\Gamma_\theta + \Gamma_\Theta}, \tag{64}$$

$$\tilde{K} = K_\theta + K_\Theta \tag{65}$$

and

$$\tilde{\lambda} = \frac{\Gamma_\theta \lambda_\Theta + \Gamma_\Theta \lambda_\theta}{\Gamma_\Theta + \Gamma_\theta}. \tag{66}$$

This has the same form as eq (7) of the main text.

$$w_2(\phi) = \frac{1}{2(\Gamma_\theta + \Gamma_\Theta)}[-\kappa_1(\phi) w_1(\phi) + w_1(\phi)^2 + \kappa_2(\phi)], \tag{67}$$

where

$$\kappa_1(\phi) = (\Gamma_\theta K_\theta + \Gamma_\Theta K_\Theta) + \frac{1}{2\Gamma}[\Delta\mu(1 - \lambda_\theta \cos(2\phi))(\zeta_2 - \zeta_1 \cos(2\phi)) + \{(\lambda_\theta - \lambda_\Theta)\cos(2\phi)\}^2] \tag{68}$$

and

$$\kappa_2(\phi) = \Gamma_\theta \Gamma_\Theta K_\theta K_\Theta + \frac{1}{2\Gamma}[\Gamma_\Theta K_\Theta \Delta\mu(1 - \lambda_\theta \cos(2\phi))(\zeta_2 - \zeta_1 \cos(2\phi)) + \tilde{K}\{\Gamma_\theta(1 - \lambda_\Theta \cos(2\phi))^2 + \Gamma_\Theta(1 - \lambda_\theta \cos(2\phi))^2\}] \tag{69}$$

$w_2(\phi)$ is positive for all $\phi$ for a large range of parameters, and its value can again be controlled by modifying the properties of the passive liquid crystal. When $w_1 < 0$ and $w_2 > 0$, patterns with a length-scale $\equiv \sqrt{w_2/w_1}$ are formed, as we pointed out in the main text.

The discussion presented here implies that the long wavelength physics of living liquid crystals is described by the theory presented in the main text. It is generally difficult to accurately measure the effective material parameters of bacteria. However, our development in this section offers an way to do so. Since the length-scale of the patterns formed depends on both the material parameters of the bacteria and those of the passive nematic, which can be characterised well, one can estimate the bacterial parameters by impregnating different passive liquid crystals with distinct, but known, parameters with the same concentration of bacteria and fitting the length-scales of the patterns obtained using our expression above. Once the bacterial parameters have been estimated this way, our prediction regarding enhanced stability can be explicitly tested by judiciously choosing a passive liquid crystal with parameter values such that $|\tilde{\lambda}| < 1$.

---

* ananyo.maitra@u-psud.fr
† martin.lenz@u-psud.fr

[1] M. C. Marchetti et al., Rev. Mod. Phys **85**, 1143 (2013)
[2] H. Stark, T. C. Lubensky, Phys. Rev. E **67**, 061709 (2003)
[3] S. Mishra, R. A. Simha, S. Ramaswamy, J. Stat. Mech. Theor. Exp. **2010**, P02003 (2010)
[4] S. Ostlund, J. Toner, A. Zippelius, Ann. Phys. **144**, 345 (1982)
[5] R. A. Simha, S. Ramaswamy, Phys. Rev. Lett. **89**, 058101 (2002)
[6] H.A. Stone, in Nonlinear PDEs in Condensed Matter and Reactive Flows, NATO Science Series C: Mathematical and Physical Sciences, **569**, H. Berestycki and Y. Pomeau eds., Kluwer Academic, Dordrecht, The Netherlands (2002); A. Oron, S.H. Davis, S.G. Banko , Rev. Mod. Phys. **69**, 931 (1997)
[7] L. Pismen, Phys. Rev. E **88**, 050502 (2013)
[8] L. Giomi et al., Phil. Trans. R. Soc. A **372**, 20130365 (2014)
[9] S. Shankar, S. Ramaswamy, M. C. Marchetti, arXiv: 1710.05400
[10] Zhou et al., Proc. Natl. Acad. Sci. USA **111**, 1265 (2014)
